# Supplementary material for: Discovering Hidden Physics Behind Transport Dynamics
Source: arXiv:2011.12222 source file (2021-03-29)
Supplement: Supplementary file 1 [file math.tex]

%%%%%%%%%%%%%%%%%%%%%%%%%%%%%%%%%%%

\section{Mathematical Preliminaries}
\label{sec: preliminaries}

\begin{itemize}

\item Gradient. In the 3D Cartesian coordinate system with a Euclidean metric, the gradient of a scalar function $f(x_1, x_2, ..., x_n)$, if it exists, is given by:
\begin{equation}
\nabla f = \frac{\partial f}{\partial x} \mathbf{i} + \frac{\partial f}{\partial y} \mathbf{j} + \frac{\partial f}{\partial z} \mathbf{k},
\label{eq: gradient}
\end{equation}
where $\mathbf{i}, \mathbf{j}, \mathbf{k}$ are the standard unit vectors in the directions of the $x, y, z$ coordinates respectively.

\item Divergence. In 3D Cartesian coordinates, the divergence of a continuously differentiable vector field $\mathbf{F} = F^x\mathbf{i} + F^y\mathbf{j} + F^z\mathbf{k}$ is defined as the scalar-valued function:
\begin{align}
\nabla\cdot\mathbf{F} &= \left( \frac{\partial}{\partial x}, \frac{\partial}{\partial y}, \frac{\partial}{\partial z} \right) \cdot (F^x, F^y, F^z) \nonumber \\
&= \frac{\partial F^x}{\partial x}+\frac{\partial F^y}{\partial y}+\frac{\partial F^z}{\partial z}.
\label{eq: divergence}
\end{align}

\item Laplacian. The Laplace operator is defined as the divergence of the gradient. I.e., for a twice-differentiable real-valued function $f$, its Laplacian is defined by:
\begin{equation}
\Delta f = \nabla^2 f = \nabla \cdot \nabla f 
\end{equation}

\item Curl. In 3D Cartesian coordinates, the curl of a vector field $\mathbf{F} = F^x\mathbf{i} + F^y\mathbf{j} + F^z\mathbf{k}$ is computed by:
\begin{align}
\nonumber \nabla \times \mathbf{F} &=
\begin{vmatrix} 
\mathbf{i} & \mathbf{j} & \mathbf{k} \\[5pt]
{\dfrac{\partial}{\partial x}} & {\dfrac{\partial}{\partial y}} & {\dfrac{\partial}{\partial z}} \\[10pt]
F^x & F^y & F^z 
\end{vmatrix}\\[1ex]
&= \left(\frac{\partial F^z}{\partial y} - \frac{\partial F^y}{\partial z}\right) \mathbf{i} + \left(\frac{\partial F^x}{\partial z} - \frac{\partial F^z}{\partial x} \right) \mathbf{j} + \left(\frac{\partial F^y}{\partial x} - \frac{\partial F^x}{\partial y} \right) \mathbf{k} \nonumber\\[1ex] 
&= \bigg[
\frac{\partial F^z}{\partial y} - \frac{\partial F^y}{\partial z}, \,
\frac{\partial F^x}{\partial z} - \frac{\partial F^z}{\partial x}, \,
\frac{\partial F^y}{\partial x} - \frac{\partial F^x}{\partial y}
\bigg]^T.
\label{eq: curl3D}
\end{align}

Curl of a 2D vector, $\mathbf{F} = F^x\mathbf{i} + F^y\mathbf{j}\,(+\,0\,\mathbf{k})$, could be expressed in the same manner:
\begin{equation}
\nabla \times \mathbf{F} =
\begin{vmatrix} 
\mathbf{i} & \mathbf{j} & \mathbf{k} \\[5pt]
{\dfrac{\partial}{\partial x}} & {\dfrac{\partial}{\partial y}} & {\dfrac{\partial}{\partial z}} \\[10pt]
F^x & F^y & 0 
\end{vmatrix}
= \bigg[
0, \, 0, \, \frac{\partial F^y}{\partial x} - \frac{\partial F^x}{\partial y}
\bigg]^T.
\label{eq: curl2D}
\end{equation}

Therefore, for a random continuous field, we clearly have
\begin{equation}
\nabla \cdot (\nabla \times \mathbf{F}) = 0,
\label{eq: div-free property}
\end{equation}
i.e., the curl of any continuous field is \textit{divergence-free} (a.k.a. \textit{incompressible} in fluid mechanics) by definition.

\item $L^p$ space: space of measurable functions for which the $p$-th power of the function absolute value is Lebesgue integrable, where functions which agree almost everywhere are identified. Specifically, let $1 \leq p < \infty$ and $(\Omega, \Sigma, \mu)$ be a measure space, $L^p(\Omega)$ space is the set of all measurable functions from whose absolute value raised to the $p$-th power has a finite integral, i.e.,
\begin{equation}
\|f\|_p \equiv \left( \int_{\Omega} |f|^p\;\mathrm{d}\mu \right)^{1/p}<\infty
\end{equation}

\end{itemize}

%%%%%%%%%%%%%%%%%%%%%%%%%%%%%%%
