# Supplementary material for: Discovering Hidden Physics Behind Transport Dynamics
Source: arXiv:2011.12222 source file (2021-03-29)
Supplement: Supplementary file 2 [file perfusion.tex]

\section{Perfusion Parameters Maps}
\label{sec: perfusion}

\subsection{Convert Measured Signal to Contrast Agent Concentration}
\cite{andreas2011perfusion}
\begin{itemize}
	\item CT perfusion: contrast agent concentration value $c(t)$ is proportional to the measured X-ray attenuation value $\mu (t)$. 
	\begin{equation}
	c(t) = k_{\text{ct}}(\mu (t) - \mu (t_0)), \quad k_{\text{ct}} \in \mathbb{R}.
	\end{equation}
	\item MR perfusion: nonlinear relation between measured signal $s(t)$ and concentration value $c(t)$:
	\begin{equation}
	c(t) = -\frac{k_{\text{mr}}}{TE}ln(\frac{s(t)}{s(t_0)}), \quad k_{\text{mr}} \in \mathbb{R}.
	\end{equation}
\end{itemize}

\subsection{Gamma Fitting for Time-Concentration Curve}
\cite{calamante2013aif}
\begin{itemize}
	\item Bolus recirculation \& noise. 
	\begin{figure}[h]
		\centering
		\includegraphics[width=0.6\linewidth]{fig/recirc.png}
		\caption{Bolus Recirculation}
	\end{figure}
    \item Gamma-variate function: focus on modeling the {\bf{first passage}}. ($BAT$: bolus arrival time)
    \begin{equation}
    C(t) = A\times (t - BAT)^B \times e^{-(t - BAT)/C}
    \end{equation}
\end{itemize}

\subsection{Perfusion Parameters Using Deconvolution}
\cite{calamante2013aif}
\begin{itemize}
	\item CBV: the amount of contrast agent passed through a specific position (voxel) $u$ w.r.t the total amount of contrast measured at the
feeding arterial vessel $C_{\text{aif}}$ (i.e., arterial input function \cite{peruzzo2011aif}):
	\begin{equation}
	CBV = \frac{\int_{t = 0}^{\infty}C(u, t)dt}{\int_{t = 0}^{\infty}C_{\text{aif}}(t)dt}
	\end{equation}
	
	\item TTP: time taken for $C(u)$ to reach maximum.
	
	\item CBF: 
	\begin{equation}
	C(u, t) = CBF\cdot C_{\text{aif}}(t)\ast R(t) = CBF\cdot \int_{0}^{t}C_{\text{aif}}(t')R(t-t')dt'
	\end{equation}
	\begin{equation}
	C(u, t_j) = \delta t \cdot CBF \cdot \sum_{i=0}^{n-1} C_{\text{aif}}(t_i) \cdot R(t_j - t_i),
	\end{equation}
	$R(t)$: residue function, fraction of injected contrast agent still present in
the vasculature at $t$ ($R(0)=1$).

	Matrix (Toeplitz matrix) form:
	
	\begin{align}
	& \begin{bmatrix}
	C(u, t_0) \\
	C(u, t_1) \\
	\vdots\\
	C(u, t_{n-1}) \\
	\end{bmatrix}
	=
	\delta t \cdot CBF \cdot \nonumber \\
	&  \begin{bmatrix}
	C_{\text{aif}}(t_0) & 0 & \dots & 0 \\
	C_{\text{aif}}(t_1) & C_{\text{aif}}(t_{0}) & \dots & 0  \\
	\vdots & \vdots & \ddots & \vdots \\
	&  C_{\text{aif}}(t_{n-1}) & C_{\text{aif}}(t_{n-2}) & \dots & C_{\text{aif}}(t_0)
	\end{bmatrix}  \cdot
	\begin{bmatrix}
	R(u, t_0) \\
	R(u, t_1) \\
	\vdots\\
	R(u, t_{n-1}) \\
	\end{bmatrix}
	\label{svd}
	\end{align}
	
	{\bf{Solve $\bf{R(t)}, \,CBF$}}: inverse matrix problem
	\begin{itemize}
		\item SVD-based: standard SVD, block-circulant SVD \cite{ostergaard2003svd,andreas2011perfusion} (Bolus arrival timing-insensitive: deals with bolus delay, dispersion)
		\begin{figure}[h]
			\centering
			\includegraphics[width=0.8\linewidth]{fig/params.png}
			\caption{Perfusion Parameters \cite{scalzi2016perfusion}}
		\end{figure}
	    \item Other deconvolution techniques \cite{ostergaard1996cnf}.
	\end{itemize}
    \item MTT: 
    \begin{itemize}
    	\item $CBV/CBF$;
    	\item $\int_{t = 0}^{\infty}R(t)dt/R_{max}$ $\Rightarrow$ $CBF = CBV / MTT$.
    \end{itemize}
\end{itemize}
