# Supplementary material for: Discovering Hidden Physics Behind Transport Dynamics
Source: arXiv:2011.12222 source file (2021-03-29)
Supplement: Supplementary file 3 [file app_2d_demo.tex]

\section{Simulation: Anisotropic Flying Points}
\label{app: 2d_demo}
