# Supplementary material for: Discovering Hidden Physics Behind Transport Dynamics
Source: arXiv:2011.12222 source file (2021-03-29)
Supplement: Supplementary file 4 [file app_results.tex]

\section{Additional Results for Sec.~\ref{exp: ixi}: Brain Advection-Diffusion}
\label{app: ixi_results}
 
\input{sub/appendix/fig/ixi_plt}

\section{Additional Results for Sec.~\ref{exp: ixi}: ISLES2017 Brain Perfusion}
\label{app: isles_results} 

\input{sub/appendix/fig/isles_plt}
