# Supplementary material for: Discovering Hidden Physics Behind Transport Dynamics
Source: arXiv:2011.12222 source file (2021-03-29)
Supplement: Supplementary file 5 [file exp_setting.tex]

\section{Experimental Settings}
\label{sec: settings}
