# Supplementary material for: Discovering Hidden Physics Behind Transport Dynamics
Source: arXiv:2011.12222 source file (2021-03-29)
Supplement: Supplementary file 7 [file app_adv_free-old.tex]

\section{Theorem 1: Divergence-free Vector Representation by the Curl of Potentials}
\label{app: proof_div_free}

{\it
\noindent For any vector field $\mathbf{V} \in L^p(\Omega)^d$ on a bounded domain $\Omega\subset\mathbb{R}^d$ with smooth boundary $\partial \Omega$. If $\mathbf{V}$ satisfies $\nabla \cdot \mathbf{V} = 0$, there exists a potential $\boldsymbol{\Psi}$ in $L^p(\Omega)^{\alpha}$ such that ($\alpha = 1$ when $d = 2$, $\alpha = 3$ when $d = 3$)
\begin{equation}
\mathbf{V} = \nabla \times \boldsymbol{\Psi}, \quad \boldsymbol{\Psi} \cdot \mathbf{n}\big|_{\partial \Omega} = 0,\, \boldsymbol{\Psi} \in L^{p}(\Omega)^{\alpha}.
\label{app_eq: repre_v}
\end{equation}
Conversely, for any $\boldsymbol{\Psi}\in L^p(\Omega)^{\alpha}$, $\nabla \cdot \mathbf{V} =\nabla \cdot (\nabla \times \boldsymbol{\Psi})= 0$.  
}

%\input{sub/appendix/fig/HHD}

\begin{proof}
Start from the general sufficiently smooth vectors in $\mathcal{H}(\Omega)$, Helmholtz-Hodge decomposition theorem \cite{maria2003hhd} ensures the existence of its divergence-free part:
\begin{theorem}[Helmholtz-Hodge Decomposition (HHD)] A sufficiently smooth vector field $\mathbf{V} \in \mathcal{H}(\Omega)$, defined on a Lipschitz domain $\Omega \subset \mathbb{R}^d$ with smooth boundary $\partial \Omega$, can be uniquely decomposed in a pure gradient field and a divergence-free vector
\label{thm: hhd}
\begin{equation}
\mathbf{V} = \nabla p + \mathbf{u}, \quad p \in \Omega,\, \mathbf{u} \in \mathcal{H}_{{\text{div}}}(\Omega).
\end{equation}
\end{theorem}
\begin{proof}
We give a brief proof here of HHD's existence, orthogonality and uniqueness for self-containness. Please refer to \cite{maria2003hhd} for detailed and alternative proofs accounting for various expressions and boundary conditions.
~\\ \vspace{-5mm}
\begin{itemize}
\item \textit{Orthogonality}. Since $\mathbf{u} \cdot \nabla p = \nabla \cdot (p \mathbf{u}) - (\nabla \cdot \mathbf{u})p$ and $\nabla \cdot \mathbf{u} =0$ by definition, hence,
\begin{align}
\int_{\Omega} \mathbf{u} \cdot \nabla p \, dx &= \int_{\Omega} \nabla \cdot (p \mathbf{u}) \, dx \quad~~ \text{($\nabla \cdot \mathbf{u} = 0$ in Eq.~(\ref{eq: div_free_space}))} \nonumber \\
&= \int_{\partial \Omega} p \mathbf{u} \cdot \mathbf{n} \, dx ~~~~~~~~ \text{(Divergence theorem)}\nonumber \\[1ex]
&=0. \quad\quad\quad\quad~~~~ \text{($\mathbf{u} \cdot \mathbf{n}|_{\partial \Omega} = 0$ in Eq.~(\ref{eq: div_free_space}))}
\label{eq: orthog}
\end{align}

\item \textit{Uniqueness}. If we have $\mathbf{V} = \nabla p_1 + \mathbf{u}_1 =  \nabla p_2 + \mathbf{u}_2$, hence $\nabla (p_1 - p_2) + (\mathbf{u}_1 - \mathbf{u}_2) = 0 $, which leads to the identity
\begin{align}
0 & = \int_{\Omega} \{ (\mathbf{u}_1 - \mathbf{u}_2) \cdot \nabla (p_1 - p_2) + \| \mathbf{u}_1 - \mathbf{u}_2 \|^2 \} \, dx  \nonumber \\
& =  \int_{\Omega} \| \mathbf{u}_1 - \mathbf{u}_2 \|^2 \, dx. \quad~~~~ \text{(Orthogonality in Eq.~(\ref{eq: orthog}))}
\end{align}
Hence $\mathbf{u}_1 \equiv \mathbf{u}_2 $, and it naturally follows $\nabla p_1 \equiv \nabla p_2$.

\item \textit{Existence}. Given a vector $\mathbf{V} \in L^2(\Omega)^d$, we consider the system with Neumann boundary condition:
\begin{equation}
\Delta p = \nabla \cdot \mathbf{V}, \quad s.t. \quad \frac{\partial p}{\partial \mathbf{n}}|_{\partial \Omega} = \mathbf{V} \cdot \mathbf{n}.
\label{eq: neumann_system}
\end{equation}
Since the solution to Eq.~(\ref{eq: neumann_system}) exists and is unique up to the addition of a constant to $p$ %\cite{courant2007math}
, the solution $p$ explicitly leads to $\mathbf{u} = \mathbf{V} - \nabla p \in \mathcal{H}_{\text{div}}(\Omega)$.
\end{itemize}
\end{proof}

Theorem \ref{thm: hhd} can be interpreted as a mapping $\mathbb{P}$, which uniquely projects the smooth vector field $\mathbf{V}$ to its divergence-free part $\mathbf{u}$ by $\mathbb{P}\mathbf{V} = \mathbf{u}$, and representing $\mathbf{V}$ as $\mathbf{u}$ plus its orthogonal complement ($\nabla p$) (See Fig. \ref{fig: hhd}). Therefore, it is natural to derive the following conclusion for the divergence-free subset $ \mathcal{H}_{{\text{div}}}(\Omega) \subset \mathcal{H}(\Omega)$:
\begin{corollary}
$\mathbb{P}$ is an identical mapping on $H_{\text{div}}(\Omega)$. I.e, for $\forall \mathbf{V} \in \mathcal{H}_{{\text{div}}}(\Omega)$, $\mathbb{P} \mathbf{V} = \mathbf{V}$.
\label{thm: equi_div_free}
\end{corollary}

Meanwhile, for special cases as $\Omega \in \mathbb{R}^2$ or $\mathbb{R}^3$, $\mathcal{H}_{\text{div}}(\Omega)$ is equivalent to the curl of potential space \cite{dubois1990div_free}. 
\begin{align*}
& \quad \mathcal{H}_{\text{div}}(\Omega) \equiv \{  \mathbf{u} = \nabla \times \psi \in L^2(\Omega)^2: \psi \in L^2(\Omega)^1 \}, \, \Omega \in \mathbb{R}^2; \\
& \quad \mathcal{H}_{\text{div}}(\Omega) \equiv \{  \mathbf{u} = \nabla \times \boldsymbol{\Psi} \in L^d(\Omega)^3: \boldsymbol{\Psi} \in L^2(\Omega)^3 \}, \, \Omega \in \mathbb{R}^3.
\end{align*}

Combining with Corollary \ref{thm: equi_div_free}, we arrive at the following conclusions for smooth divergence-free velocity fields in 2D and 3D:\\~\\%, by which Req.~\ref{div_free req: 1} and Req.~\ref{div_free req: 2} are satisfied.
{\bf{[2D]}}
\begin{itemize}
\item {\textbf{Equivalence between spaces}}. The space of sufficiently smooth divergence-free vector fields $\mathcal{H}_{\text{div}}(\Omega \subset \mathbb{R}^2)$ is equivalent to the curl of scalar potential space:
\begin{align}
\quad \mathcal{H}_{\text{div}}(\Omega) & \equiv \big\{\mathbf{u} \in \mathbb{P} \mathcal{H}(\Omega) \,\big|\, \mathbf{u} \cdot \mathbf{n}|_{\partial \Omega} = 0 \big\} \nonumber \\
& \equiv \big\{  \mathbf{u} = \nabla \times \psi \in L^2(\Omega)^2 \,\big|\, \psi \in L^2(\Omega)^1 \big\}.
\end{align}
\item {\textbf{Surjective mapping}}. Any $\mathbf{V} \in \mathcal{H}_{\text{div}}(\Omega \subset \mathbb{R}^2)$ can be represented in the form:
\begin{align}
& \mathbf{V} = \nabla \times \psi, \quad \psi \in L^2(\Omega)^1,\, \Omega \subset \mathbb{R}^2,  \nonumber \\
& s.t. 
\begin{cases}
   \nabla \cdot \mathbf{V} = 0 \text{~on~} \Omega, \\
   \mathbf{V} \cdot \mathbf{n}|_{\partial \Omega} = 0. 
\end{cases}
\end{align}

\end{itemize}

{\bf{[3D]}}
\begin{itemize}
\item {\textbf{Equivalence between spaces}}.  The space of sufficiently smooth divergence-free vector fields $\mathcal{H}_{\text{div}}(\Omega \subset \mathbb{R}^3)$ is equivalent to the curl of vector potential space:
\begin{align}
\quad \mathcal{H}_{\text{div}}(\Omega) & \equiv \big\{\mathbf{u} \in \mathbb{P} \mathcal{H}(\Omega) \,\big|\, \mathbf{u} \cdot \mathbf{n}|_{\partial \Omega} = 0 \big\} \nonumber \\
& \equiv \big\{  \mathbf{u} = \nabla \times \boldsymbol{\Psi} \in L^2(\Omega)^3 \,\big|\, \boldsymbol{\Psi} \in L^2(\Omega)^3 \big\}.
\end{align}

\item {\textbf{Surjective mapping}}. Any $\mathbf{V} \in \mathcal{H}_{\text{div}}(\Omega \subset \mathbb{R}^3)$ can be represented in the form:
\begin{align}
& \mathbf{V} = \nabla \times \boldsymbol{\Psi}, \quad \boldsymbol{\Psi} \in L^2(\Omega)^3,\, \Omega \subset \mathbb{R}^3, \nonumber \\
& s.t. 
\begin{cases}
   \nabla \cdot \mathbf{V} = 0 \text{~on~} \Omega, \\
   %\nabla \cdot \mathbf{\boldsymbol{\Psi}} = 0 \text{~on~} \Omega, \\
   \mathbf{V} \cdot \mathbf{n}|_{\partial \Omega} = 0.
\end{cases}
\end{align}

\end{itemize}

The divergence-free property of curl of potential fields ensures Req.~(\ref{div_free req: 1}), and the surjective mappings between potential fields to vector field further satisfies Req.~(\ref{div_free req: 1}). The above conclusions directly lead to Theorem 1.
\end{proof}
